# Supplementary material for: Conversational Question Answering with Reformulations over Knowledge Graph
Source: arXiv:2312.17269 source file (2024-03-29)
Supplement: Supplementary file 1 [file 09Appendix.tex]

\section{Appendix}

\subsection{Dataset}
We use two datasets in the experiments: ConvQuestions ~\cite{convex} and ConvRef ~\cite{conquer}.
ConvQuestions contains a total of 6,720 conversations, each with 5 turns, but no human writing reformulations are provided in this dataset.
ConvRef contains a total of 6,720 conversations, each with 5 turns, and each question has several human writing reformulations.
All the conversations in ConvQuestions and ConvRef belong to one of the five domains: "Books", "Movies", "Soccer", "Music", and "TV Series".
Each domain contains 1344 training conversations, 448 validation conversations and 448 test conversations. 
The statistics of these datasets are shown in Table ~\ref{datasets}.

\begin{table}[h]
	\centering
	\caption{Summary of datasets.}
	\begin{tabular}{|c|c|c|c|c|c|c|}
	\hline
	Dataset          & Train & Valid & Test \\ \hline
	{\tt ConvQA} & 6,720   &  2,240    & 2,240    \\ 
	{\tt ConRef} & 6,720   & 2,240      & 2,240    \\ \hline
 %    Domain          & Train & Valid & Test  \\ \hline
	% {\tt ConRef} Movies & 1344   & 448       & 448    \\ 
	% {\tt ConRef} TV Series & 1344   & 448       & 448   \\ 
	% {\tt ConRef} Music & 1344  & 448       & 448   \\ 
 %    {\tt ConRef} Books & 1344   & 448      & 448    \\ 
	% {\tt ConRef} Soccer & 1344   & 448       & 448    \\ \hline
	\end{tabular}
	\label{datasets}
\end{table}

\subsection{Experiment Setting}

All experiments are conducted on a machine with an Intel(R) Xeon(R) Gold 6240R CPU, 1510 GB memory, and an NVIDIA-SMI Tesla V100-SXM2 GPU.
When using ComplEx to learn the KG embeddings, we use a hidden dimension of 200 and train for 100 epochs with a batch size of 256. For \myModel, we set the hidden dimension to 200, the batch size to 12, the learning rate to 0.00002, and train for 20 epochs, storing checkpoints along the way. The Adam optimizer ~\cite{adam} is used with fixed weight decay of 1.0.
For the pre-trained BERT model, we set the maximum sentence size to 64 tokens, padding if necessary. The token dimension is 128.
%Table ~\ref{Hyperparameters} summarizes the hyperparameters used in the experiments.

\subsection{Baselines}

We compare the performance of our method, \myModel, with four baselines:
\begin{itemize}
    \item \textbf{Convex} ~\cite{convex}: This method detects answers to conversational utterances over KGs in a two-stage process based on graph expansion. It first detects so-called frontier nodes that define the context at a given turn and then finds high-scoring candidate answers in the vicinity of the frontier nodes.
    \item \textbf{Conqer} ~\cite{conquer}: This is the current state-of-the-art baseline. It uses RL with reformulations to find answers in the KG. %However, unlike \myModel, 
    It employs multiple agents to find multiple answers for each question and ranks these answers in the end.
    \item \textbf{OAT} ~\cite{OAT}: This Transformer-based model takes a JSON-like structure as input to generate a Logical Form (LF) grammar that can model a wide range of queries on the graph. It finds answers by applying the LF.
    \item \textbf{Focal Entity} ~\cite{lan-jiang-2021-modeling}: This is a novel graph-based model that captures transitions of focal entities and applies a graph neural network to derive a probability distribution of focal entities for each question. The probability distribution is then combined with a standard KBQA module to rank answers. 
\end{itemize}
Note that Convex and Conqer utilize named entity recognition (NER) to identify topic entities in a question. Since we assume that the topic entity of $q_1$ is {given}, in order to ensure a fair comparison, we revise the NER method in Convex and Conqer so that it returns the main topic entity of $q_1$ directly.

\subsection{The effectiveness of the unique relation embedding}

We also test the effectiveness of using a unique edge embedding in the action space with reinforcement learning.
4 reformulations are used in the experiments, and the results are shown in Table ~\ref{edge_emb}. In this table, " \myModel\ -" denotes \myModel\ without using a unique edge embedding. 
As we can see, using a unique edge embedding improves the question answering performance by an average of 2.2\%. 

\begin{table}[H]
	\centering
	\caption{The effectiveness of the unique edge embedding.}
 \scalebox{0.8}{
	\begin{tabular}{|c|c|c|c|c|c|c|}
	\hline
	Model          &  P@1 & Hit@3 & Hit@5  & Hit@8 & MRR   \\ \hline
	\myModel\ -  & 0.227  &  0.396 & 0.469 & 0.507 & 0.330 \\ \hline
	\rowcolor{lightgray} \myModel\ & 0.265  & 0.404 &  0.477 & 0.526  & 0.353 \\ \hline
	\end{tabular}
 }
	\label{edge_emb}
\end{table}

\subsection{The effectiveness of the topic entity selector.}

The topic entity selector is pre-trained using the training data
%, and the teacher model is used to encode the input questions and reformulations during training. Note that a new teacher model will be retrained with the RL-based QA model after the topic entity selector is pre-trained. 
After pre-training, the results of the accuracy for the classifier is 83.2\%. We find that the classifier has a relatively high accuracy.
